# Supplementary material for: Beyond Winning Strategies: Admissible and Admissible Winning Strategies for Quantitative Reachability Games
Source: arXiv:2408.13369 source file (2025-06-06)
Supplement: Supplementary file 1 [file hopeful_admissible.tex]

\subsection{Hopeful Admissible Strategies}

In this section, I will brainstorm on the desired behavior from a stronger notion of admissible strategies.

What - We want a stronger notion of admissible strategies. 

How - The are a bunch of ways to do it.

\begin{table*}[t!]
    \centering
    \resizebox{1\textwidth}{!}{%
    \begin{tabular}{c||c|c|c|a|c}
        \toprule
        & Hopeful-admissible  & Hopeful-admissible  & Admissible-Winning & Admissible-Winning & Admissible (org.) \\ 
         Property & ($\sco$ + $\wcoop$) & ($\wcoop$) & ($\wcoop$)& ($\sco$-M + $\wcoop$) & ($\sco$ + $\wcoop$) \\
         \hline \hline 
         Asmp. on Env & \cmark & \cmark & \xmark & \xmark & \xmark \\
         Winning (from $V_{win}$) & \cmark  & \cmark & \cmark & \cmark & \xmark \\
         State-Value Preserving & \cmark (Trivial) & \cmark (Trivial) & \cmark & \cmark & \xmark \\
          Memory & Unbounded & Memoryless & Memoryless & Unbounded & Unbounded \\
          Algo. - Unroll & \cmark & \xmark & \xmark & \cmark & \cmark \\
        \bottomrule
    \end{tabular}
    }
    \caption{In the hopeful case, we make a rationality assumption on the Env player.}
    \label{tab: hopeful_sec_table}
\end{table*}

\subsubsection{Approach}

We have that admissible strategies are finite-memory (history-dependent) and are overly optimistic. For a strategy to be admissible it has to be $\sco$ or $\wcoop$. 

$\sco$ - strongly cooperative strategy $\sigma$ where a strategy can take a riskier action (higher $\aVal(h, \sigma)$) as long there exists a lower payoff. This makes the strategy overly optimistic. $\Sigma_{adm}$ are not state value preserving because of $\sco$.

$\wcoop$ - worst-case cooperative optimal strategy $\sigma$ is a strategy where $\sigma$ ensures worst-case payoff along with the optimal cooperative value. This enforces a worst-case outcome and leaves room for cooperation.

\begin{table}[tbh!]
    \centering
    \begin{tabular}{c||c||c}
        \toprule
         Qualitative & Quantitative (Org.) & Quantitative (Hopeful) \\ \hline \hline 
           $1 \to 1$ &  $1 \to 1, \textcolor{red}{0}$ & $1 \to 1$\\
           $0 \to 0, 1$ &  $0 \to 0, 1$ & N/A \\
           $-1 \to -1$ & $ -1 \to -1$ & $-1 \to -1$\\
        \bottomrule
    \end{tabular}
    \caption{State Value preservation: In qualitative settings, an admissible strategy never decreases its value. In quantitative settings, an admissible strategy can decrease its value at the expense of lower payoff value.}
    \label{tab: my_label}
\end{table}

Solution to mitigate optimism is 

\begin{itemize}
    \item Enforce State value to never decrease in quantitative settings. This can be done by modifying the $\sco$ condition to be $$ \cVal(h, \sigma) < \aVal(h)  \wedge \aVal(h, \sigma) \neq \infty$$

    Here $\aVal(h, \sigma) \neq \infty$ should hold for all Sys player states in all prefixes $h$ of plays that start from $v \in V_{win}$.
    \item If the Env player is playing hopefully then all states in $\G$ will have a state value of 1 (ignoring $V_{los}$). Then the state value preservation happens implicitly. But, we 
\end{itemize}

\input{appendix_fig_tex/str_dominant_game}

\subsubsection{Strictly Dominant Strategy}

What if we synthesize a strictly dominant strategy. Lets take for example the game in Figure \ref{fig: str_dominant_stra_game}. For a dominant strategy to exists it needs to always do better than the other strategies, i.e.,  

$$\aVal(h) = \aVal(h, \sigma) \wedge \aVal(h) < \cVal(h, \sigma')$$

where $\sigma' \in \Sigma $ is a valid strategy at $h$ and $\sigma' \neq \sigma$. Thus, $\sigma$ strictly dominates ($\succ^{SD}$) $\sigma'$. In Figure \ref{fig: dominant_str_game}, strategy that commits to $v_0 \to v_2$ strictly dominates strategy to commits to $v_3 \to v_5$. But, if the game includes state $v_4$ then no strictly dominating strategy exists. 

\subsubsection{Dominant Strategy}

A strategy $\sigma$ is called dominant strategy iff there exists a $\sigma'$ that is being dominated. Just like admissible strategy, Dominant strategies (if they exists) are also maximal in order. We modify the original game from Figure \ref{fig: local_conds_not_sufficient}, and restrict the human to only hopeful strategies then we get the game in Figure \ref{fig: hope_dominant_str_game}. Here strategy $\sigma'$ that commit to $v_7 \to v_9$ is dominated. Although, $\sigma'$ enforces the best it can do but is not $\wcoop$. Strategy $\sigma$ that commits $v_3 \to v_5$ dominates $\sigma'$ as it is $\wcoop$. Strategy $\sigma''$ that commits to $v_7 \to v_8$ is $\sco$. Thus, for this game we have a dominant strategy.   

But, if we modify the payoff from $v_9$ and add $3$, then any strategy that commits $v_7 \to v_9$ is admissible. In fact, every strategy in the modified game is admissible. Note that there does not exist a dominated strategy. Thus, for the modified game, a dominant strategy does not exist!

\input{appendix_fig_tex/hope_dominant_fig}

\begin{itemize}
    \item Strictly Dominating strategy - too restrictive
    \item Dominant Strategy - Do not always exist.\textbf{ Do enforce reaching a goal state - this is because we are playing against an hopeful Env player.} 
\end{itemize}

\input{appendix_fig_tex/dominant_fig}

\begin{tcolorbox}[title= Question]
If you are synthesizing hopeful-Admissible winning, i.e., $\wcoop$ then are memoryless strategies sufficient, yes! - 
See Thm. \ref{thm: wcoop_memoryless}
But, to compute  Hopeful adversarial strategies for the Env player we need to keep track of the history. See our example from the old IJCAI paper - choice of Eny player at State $s_7$ depends on the history.
\end{tcolorbox}

\subsubsection{Env being hopeless}

If we are playing against a hopeless Env player, then to enforce state value preservation we can modify $\sco$, written $\sco$-M, as mentioned above to be

 $$ \cVal(h, \sigma) < \aVal(h)  \wedge \aVal(h, \sigma) \neq \infty$$

 Intuitively, for a prefix $h$ if the last state $v_s \in V_{win}$ then, the play should remain in the winning region. \textbf{By adding this constraint, we are removing some admissible strategies.} In figure \ref{fig: dominant_str_game}, including the dashed edges, an admissible strategy that follows above condition will no commit to $v_7 \to v_9$ even though the $\cVal(v_9) = 3$. While according to the original $\sco$ definition, edge $v_7 \to v_9$ does belong to admissible strategy as there exists a payoff of $3$.
