# Supplementary material for: Beyond Winning Strategies: Admissible and Admissible Winning Strategies for Quantitative Reachability Games
Source: arXiv:2408.13369 source file (2025-06-06)
Supplement: Supplementary file 2 [file nec_suff_conds_for_adm.tex]

\section{Necessary and Sufficient Conditions for Admissibility}

Attributes of admissible strategies:

\begin{itemize}
    \item Not every $\wco$ strategy is admissible.
    \item Not every admissible strategy is a winning strategy.
    \item Quantitative Admissible strategies are not State Value Preserving. This implies that we can not use algorithms developed for the qualitative-variant \cite[Abstraction based]{brenguier2015assume}, \cite[Parity Game based]{brenguier2014complexity}.
    \item Admissible strategies are not memoryless. \km{Are they finite memory or infinite memory - need to establish this}
    \item All valid edges from Sys player states in $V_{pen}$ are part of an admissible strategy. Side Note: for a valid edge $(v_s, v_e)$ if $v_s \in V_{pen} \to v_e \in V_{pen}$. This is because, the edge the Sys player can choose $v_s \to v_e$ and hence if $v_e \in  V_{win} \to v_s \in V_{win}$.  
\end{itemize}

Here are two conditions that establish if a strategy is admissible or not. 

\subsection{Are Worst-case optimal strategies always admissible? ($\wco$) - No!}

Not all $\wco$ strategies are admissible. For example, in Figure \ref{fig: wco_ex_1}, a strategy that commits to payoff of 2 from state $v_2$ is $\wco$. But, an admissible strategy from $v_2$ is to commit to 2 or go to $v_3$. Thus, both actions belong to an admissible strategy. Thus, not every admissible strategy is $\wco$. 

Intuitively, a strategy is admissible if it is playing Strongly Cooperative Optimal ($\sco$), i.e., they either ensure worst-case optimal $(\aVal(h))$ or choose a higher worst-case optimal strategy if there exists a better (lower payoff) cooperative value ($\cVal(h, \sigma)$) along this strategy.

$\mathbf{Cond. \; 1}$: $\cVal(h, \sigma) < \aVal(h)$

Further, in Figure \ref{fig: wco_ex_2}, strategy from $v_2$ that commits to 2 or goes to $v_3$ are both $\wco$. But only a strategy that commits to $v_3$ is admissible. Thus, not every $\wco$ strategy is admissible. In this example, committing to $v_3$ ``safely" maximizes the cooperative value while enforcing a worst-case optimal payoff. $\aVal(v_2, \sigma' := v_2 \to 2) = \aVal(v_2, \sigma := v_2 \to 3) = 2$ and $\cVal(v_2, \sigma) = 1$. Here $\sigma \succ \sigma'$. 

Thus, $\sigma'$ is dominated by $\sigma$ if
\begin{equation*}
    \underbrace{\aVal(h, \sigma') = \cVal(h, \sigma')}_{\text{best $\sigma'$ can do}} = \underbrace{\aVal(h, \sigma) > \cVal(h, \sigma)}_{\substack{\text{$\sigma$ ensures $\wco$ payoff but} \\ \text{$\exists$ better payoff}}}
\end{equation*}

Thus, if a strategy is worst-case cooperative optimal ($
\wcoop$), i.e., it ensures the minimum payoff the Sys player can achieve from $h$ with Env player's help while enforcing the worst-case optimal payoff value $\aVal(h)$. Thus, if $\acVal(h) = \aVal(h)$ then all $\wco$ strategies are admissible.

$\mathbf{Cond. \; 2}$: $\aVal(h) = \aVal(h, \sigma) = \acVal(h)$

Thus, to ensure a strategy $\sigma$ is admissible, it needs to be $\sco$ and $\wcoop$, i.e., 

\begin{align}
    \cVal(h, \sigma) < \aVal(h) \\
    \vee \left(\aVal(h) = \aVal(h, \sigma) \wedge \cVal(h, \sigma) = \acVal(h) \right)
\end{align}

Simplifying the above equations, we get 

\begin{align}
    \cVal(h, \sigma) < \aVal(h) \\
    \vee \aVal(h) = \aVal(h, \sigma) = \cVal(h, \sigma) = \acVal(h)
\end{align}

\subsection{Are Cooperative optimal strategies always admissible? ($\coop$) - Yes!} 

A strategy $\sigma$ where $\cVal(h, \sigma) > \aVal(h)$ is not admissible. A Cooperative Optimal strategy $\sigma$ will always be maximal in the order because it has the least payoff, i.e., for a given history $h$, $\cVal(h) \leq \aVal(h)$ and $\cVal(h, \sigma) \leq \cVal(h)$. Hence, $\cVal(h, \sigma) \leq \aVal(h)$. Thus, a cooperative optimal strategy will never satisfy $\cVal(h, \sigma) > \aVal(h)$ and hence is always admissible.

\begin{lemma}
    All $\sco$ strategies are admissible 
\end{lemma}
\begin{proof}
    A strategy $\sigma$ is not $\sco$ if $\neg (\cVal(h, \sigma) < \aVal(h))$.
\end{proof}

\begin{lemma}
    $\neg (\cVal(h, \sigma) < \aVal(h))$ is $\cVal(h, \sigma) \geq \aVal(h)$
\end{lemma}
\begin{proof}
    $\neg (\cVal(h, \sigma) < \aVal(h)) = (\cVal(h, \sigma) > \aVal(h)) \vee (\cVal(h, \sigma) = \aVal(h)) $ 
\end{proof}

\begin{lemma}
    $\neg (\aVal(h) = \aVal(h, \sigma) = \acVal(h))$ is $\text{?}$
\end{lemma}

\begin{lemma} Strategies that never reach the goal state are not admissible 
\end{lemma}
\begin{proof}
    As per our payoff definition, any play that never reaches the goal state will have a payoff of $\infty$. Contrarily, plays that are finite in length will always reach the goal state in finite steps and that the corresponding payoff will be $< \infty$. Thus, strategies ($\sigma \in \Sigma$) that never reach goal state are strictly dominated by strategies ($\sigma' \in \Sigma$) that reach a goal state at least once.
\end{proof}

\input{appendix_fig_tex/adm_in_pen}

\begin{lemma} All valid edges from Sys player states in $V_{pen}$ that stay do not transition to $V_{los}$ are NOT part of admissible strategy
\end{lemma}
\begin{proof}
   The proof is straightforward. See Figure \ref{fig: adm_in_pen}
\end{proof}

\input{appendix_fig_tex/wco_admissibility}

\subsection{Algorithm for Admissible Strategy Synthesis}

Currently, there are two proposed algorithms for synthesizing admissible strategies. 

\paragraph{Algorithm 1. - Tree Based} The algorithm is outlined in Algo. \ref{algo: naive_adm}. Given the game venue $\G$ and maximum payoff that the Sys player can expend (energy budget $B$), we construct a tree of plays $G'$ corresponding to strategy $\Sigma$ and $\Tau$ such every play that reached a goal state with payoff less than $B$ is assigned a goal state otherwise it is sink state. The strategies are then synthesized on $G'$. - Complexity - $\mathcal{O}(|V| + |E|)$.

\paragraph{Algorithm 2. - Budget Free approach} The idea for this algorithm is construct a parity automaton corresponding to all plays induced by strategy $\Sigma$ and $\Tau$. Next, we play  zero-sum game and synthesize winning strategy for the Sys player.  - Complexity of solving Pariy games - Complexity - UP and co-UP. 

\km{Work in Progress - Constructing this parity game}

\paragraph{Algorithm 3. - Online algorithm} Instead of computing the set of admissible strategies, we can modify our Problem formulation for Sys player to just play admissibly. This means that we compute the $\aVal$, $\cVal$, and $\acVal$ for every state and then
