# Supplementary material for: Beyond Winning Strategies: Admissible and Admissible Winning Strategies for Quantitative Reachability Games
Source: arXiv:2408.13369 source file (2025-06-06)
Supplement: Supplementary file 3 [file other_proofs.tex]

\section{More admissible strategy properties}

\begin{lemma}
 Given $\G$, and strategy $\sigma$ that is admissible, $\forall h \in \plays^{h}(\sigma)$ such that $\aVal(h) < \infty$, $\sigma \not\equiv \sigma_{win}$    
 \label{lem: adm_win_not_same}
\end{lemma}
\begin{proof}
    Proof by Lemma \ref{lem: quant_adm_not_val_pres}. We first observe that an optimal winning strategy $\sigma_{win}$ satisfies the condition $\aVal(h, \sigma_{win}) = \aVal(h)$. Thus, $\sigma_{win}$ enforce reaching a goal state for all Env player strategies $\tau \in \Tau$. Thus, every $\sigma_{win}$ ensures that every state for every play in $\plays^{v}(\sigma_{win})$ belongs to $V_{win}$. Hence, from Lemma \ref{lem: quant_adm_not_val_pres}, we have that not all admissible strategies are $\wco$.

    In Fig. \ref{fig: cex_adm_val_not_preserving}, a Sys player strategy that commits to $v_1$ from $v_0$ is $\wco$. Thus, actions $v_4 \to v_5$ and $v_4 \to v_7$ belong to strategy that is $\wco$. But, only action $v_4 \to v_7$ belongs to an admissible strategy as there exists a better payoff while enforcing the worst-case optimal payoff. Therefore, not every $\wco$ strategy is an admissible strategy.
\end{proof}

Thus, from Lemma \ref{lem: adm_win_not_same}, we have that admissible strategies are not equivalent to winning strategies.

\subsection{When are $\wco$ admissible?}

Another interesting characterization of admissible strategy is as follows. Given history $h$, if $\acVal(h) = \aVal(h)$, then the adversarial-cooperative value and adversarial value for $h$ are the same. This implies,  strategy $\sigma$ that is $\wco$ is also $\wcoop$. Thus, $\sigma$ that is worst-case optimal is admissible. 

\begin{lemma}
    All worst-case optimal $(\wco)$ strategies are admissible if $\acVal(h) = \aVal(h)$,  
\end{lemma}
\begin{proof}
    A strategy $\sigma$ that witnesses $\acVal(h)$ is maximal in order. There does not exist another strategy that ensures a lower payoff while being $\wco$. There might exist $\sigma'$ that achieves lower payoff against some adversary but will be receive higher payoff against another adversary, i.e., $\aVal(h, \sigma') > \aVal(h)$. Hence, $\sigma'$ does not dominate $\sigma$.
    Thus, if $\acVal(h) = \aVal(h)$, then all $\wco$ strategies are admissible. Further, if $\acVal(h) < \aVal(h)$, then a worst-case optimal strategy $\sigma$ is admissible if, and only if, $\cVal(h, \sigma) < \aVal(h)$ and $\cVal(h, \sigma)=~\acVal(h)$. 
\end{proof}
