# Supplementary material for: Beyond Winning Strategies: Admissible and Admissible Winning Strategies for Quantitative Reachability Games
Source: arXiv:2408.13369 source file (2025-06-06)
Supplement: Supplementary file 4 [file parity_automaton.tex]

\subsection{Parity Automaton Algorithm}

These are just notes. The advantage of Parity Automaton approach is that the algorithm does not need as input an energy budget (which implicitly bounds the depth of the Tree of outcomes). 

Zielonka Tree -  what and is it useful? 

\paragraph{How to convert my Game to Parity Automaton} Infinite plays of the form $\play = (V)^*(V_f)^\omega$ will have a finite payoff that. Infinite plays of the form $\play = (V)^*(V')^\omega$ where $v \notin V_f \forall v \in V'$ will have a payoff of $\infty$. 

\begin{tcolorbox}[title= Question]
  Do you need prefix independent condition to construct the parity automaton for all plays?

  \tcblower

  According to \cite[Section 5]{brenguier2016admissibility}, under prefix-independent condition, we can compute a finite set of $\aVal$, i.e., $\aValues := \{\aVal\}$. This is not necessarily true for the case of prefix-dependent payoff they consider like - Inf, Sup. While our payoff is \emph{not} prefix-independent, we can always compute a finite set of $\aVal$ associated with each state in $\G$. Further, in \cite[Section 6]{brenguier2016admissibility}, the authors mention 

  \begin{quote}
      However it seems feasible for regular payoﬀs, such as Inf, Sup, LimInf and LimSup, for which we can \emph{construct parity automata recognizing outcomes with $\Val > q \; \forall q \in \aValues$.}
  \end{quote}
\end{tcolorbox}
