# Supplementary material for: Beyond Winning Strategies: Admissible and Admissible Winning Strategies for Quantitative Reachability Games
Source: arXiv:2408.13369 source file (2025-06-06)
Supplement: Supplementary file 5 [file qual_def.tex]

\section{Clarification - Qualitative vs. Quantitative}

\subsection{Existing Qualitative Dominance Definition}

These notions are common in the Formal Methods community where the objective is Boolean and the corresponding payoff is binary (win or lose \cite{berwanger2007admissibility}). 

\begin{definition}[Dominance (Quant - very weakly dominating) \cite{benjamin2021best}]
\label{def: qual_dom}
      Given two Sys strategies $\sigma,\sigma' \in \Sigma$, we say $\sigma$ \emph{dominates} $\sigma'$, denoted by $\sigma \succeq \sigma'$, if for every env strategy $\tau \in \Tau$, $\play^{v_0}(\sigma', \tau) \models \phi \to \play^{v_0}(\sigma, \tau) \models \phi$. 
\end{definition}

Intuitively, given two strategies $\sigma$ and $\sigma'$ for the agent, we say that $\sigma$ dominates $\sigma'$ if $\sigma$ is as good $\sigma'$ for some environment strategies $\tau$. We note that Strict Dominance was \textbf{NOT} defined using the definition env. \cite{benjamin2021best,aminof2023dominant}.

\begin{definition}[Strict Dominance (Quant - weakly dominating)]
\label{def: qual_strict_dom}
      Given two Sys strategies $\sigma,\sigma' \in \Sigma$, we say $\sigma$ \emph{strictly dominates} $\sigma'$, denoted by $\sigma \succ \sigma'$, if $\sigma \succeq \sigma'$ and $\neg(\sigma' \succeq \sigma)$.
\end{definition}

We say $\sigma$ strictly dominates $\sigma'$ if it does as good as $\sigma'$ and is better than $\sigma'$ in at least one case. Note, better $\to$ reaching a goal state for Two-player Reachability games.

\begin{definition}[admissible \cite{berwanger2007admissibility}]
    A strategy is called \emph{admissible} for the Sys player if it is not \emph{dominated} ($\succ$; as per Def. \ref{def: qual_strict_dom}) by any other strategy of the Sys player. 
\end{definition}

\begin{definition}[Best-Effort \cite{benjamin2021best,aminof2023dominant,faella2009admissible}]
    A strategy is called \emph{Best-Effort} for the Sys player if it is not \emph{dominated} ($\succ$; as per Def. \ref{def: qual_strict_dom}) by any other strategy of the Sys player. 
\end{definition}

So, by definition, in Qualitative settings, both Best-Effort and Admissible strategies are equivalent \cite{benjamin2021best,aminof2023dominant}. The same is not true in the Quantitative settings.

\begin{table}[tbh!]
    \centering
    \resizebox{1\columnwidth}{!}{%
    \begin{tabular}{c||c}
        \toprule
         Qualitative & Quantitative \\ \hline \hline 
         Dominance (Def. \ref{def: qual_dom}) & Very weakly dominating (Def. \ref{def: dom_str}) \\
         strict dominance (Def. \ref{def: qual_strict_dom}) ) & weakly dominating (Def. \ref{def: dom_str})  \\
         N.A. & strictly dominating (Def. \ref{def: dom_str}) \\
         Admissible $\equiv$ BE & Admissible (BE - N.A.) \\
        \bottomrule
    \end{tabular}
    }
    \caption{Equivalent definition of dominance across qualitative \cite{benjamin2021best, berwanger2007admissibility} and quantitative papers \cite{Leyton-Brown2008, brenguier2016admissibility}}
    \label{tab:my_label}
\end{table}
