# Supplementary material for: Beyond Winning Strategies: Admissible and Admissible Winning Strategies for Quantitative Reachability Games
Source: arXiv:2408.13369 source file (2025-06-06)
Supplement: Supplementary file 6 [file inf_non_dom_chain.tex]

\subsection{Non-Dominated weak dominance chain}

Since, we do not have  negative weights in our game, our graph does no have Negative Cycles (NC), i.e., the payoff is never $\not< 0$. Thus, the Env player can not trap the Sys player in a NC cycle \cite{brihaye2017pseudopolynomial}. Thus, using the similar argument as \cite[Example 9]{brenguier2016admissibility}, in our games, there does not exist an infinite dominance chain such that $\sigma^{\infty}$ (infinite memory) weakly dominates $\sigma^{< \infty}$.

\begin{figure}[t!]
    \centering
    \begin{subfigure}[t]{0.49\linewidth}
    \resizebox{\linewidth}{!}{%
        \centering
        \begin{tikzpicture}[
        ->,>=stealth',shorten >=1pt,shorten <=1pt,auto,node distance=1cm,
        every loop/.style={looseness=6},
        initial text={},
        el/.style={font=\scriptsize},
        every fit/.style={draw,densely dotted,rectangle},
        inner sep=2mm,
        loopright/.style={loop,looseness=6,out=-45, in=45},
        loopleft/.style={loop,looseness=6,out=135, in=225},
        loopabove/.style={loop,looseness=6,out=45, in=135},
        loopbelow/.style={loop,looseness=6,out=-135, in=-45},
        ]
        \tikzstyle{every state}=[node distance=1.4cm,minimum size=7mm, inner sep=1pt]; 
        \node[state, initial] (v0) {$v_0$};
        \node[state, rectangle, right of=v0] (v1) {$v_1$};
        \node[state, accepting, right of=v1] (v2) {$v_2$};
        \node[state, rectangle, above of=v0] (v3) {$v_3$};
        \path[->]
            (v0) edge[bend left] node {1} (v1)
            (v1) edge[bend left] node {0} (v0)
            (v1) edge node[below] {0} (v2)
            (v2) edge[loop] node[above] {0} (v2)
            (v0) edge node {10} (v3)
            (v3) edge node {0} (v2);
        \end{tikzpicture}
        }
    \caption{}
    \label{fig: inf_dom_ex_1}
    \end{subfigure}%
    ~
    \begin{subfigure}[t]{0.49\linewidth}
    \resizebox{\linewidth}{!}{%
        \centering
        \begin{tikzpicture}[
        ->,>=stealth',shorten >=1pt,shorten <=1pt,auto,node distance=1cm,
        every loop/.style={looseness=6},
        initial text={},
        el/.style={font=\scriptsize},
        every fit/.style={draw,densely dotted,rectangle},
        inner sep=2mm,
        loopright/.style={loop,looseness=6,out=-45, in=45},
        loopleft/.style={loop,looseness=6,out=135, in=225},
        loopabove/.style={loop,looseness=6,out=45, in=135},
        loopbelow/.style={loop,looseness=6,out=-135, in=-45},
        ]
        \tikzstyle{every state}=[node distance=1.4cm,minimum size=7mm, inner sep=1pt]; 
        \node[state, initial] (v0) {$v_0$};
        \node[state, rectangle, right of=v0] (v1) {$v_1$};
        \node[state, accepting, right of=v1] (v2) {$v_2$};
        \node[state, rectangle, above of=v0] (v3) {$v_3$};
        \path[->]
            (v0) edge[bend left] node {0} (v1)
            (v1) edge[bend left] node {0} (v0)
            (v1) edge node[below] {2} (v2)
            (v2) edge[loop] node[above] {0} (v2)
            (v0) edge node {10} (v3)
            (v3) edge node {0} (v2);
        \end{tikzpicture}
        }
    \caption{}
    \label{fig: inf_dom_ex_2}
    \end{subfigure}%
    \caption{Infinite dominance chain example (a) (b)}
\end{figure}

In Figure \ref{fig: inf_dom_ex_2} if $\sigma^{k}$ is a strategy to loop k times before committing to $v_3$ then $\sigma^{k+1}$ weakly dominates $\sigma^{k}$ as it can ensure that same payoff in worst -case scenario but better payoff if the Env player is cooperative. This is not the case in Figure \ref{fig: inf_dom_ex_1}. This seems to be due to the property that our payoff is monotonically increasing.
