# Supplementary material for: Beyond Winning Strategies: Admissible and Admissible Winning Strategies for Quantitative Reachability Games
Source: arXiv:2408.13369 source file (2025-06-06)
Supplement: Supplementary file 7 [file regret_min_adm.tex]

\subsection{Regret Minimizing Admissible strategy}

This is a just a brainstorming section. We could the admissibility definition as follows. 

Idea: Admissible strategies are too optimal. We need to way to mitigate the optimism. We could use the definition of regret (worst that can happen under $\sigma$ - best that could have happened under $\sigma'$)
